# Supplementary material for: Layer Pruning with Consensus: A Triple-Win Solution
Source: arXiv:2411.14345 source file (2024-11-21)
Supplement: Supplementary file 1 [file Appendix_CopiaConflitoIan.tex]

\newpage
\section{Appendix}\label{sec:app}
\subsection{Technical Details Involving Layer Pruning}\label{sec:technical_issues}
%\todo{Adaptar essa descrição como está no problem statement. La eh N e nao F.}
Let $\mathcal{N}$ be a network composed of $L$ layers. We can express the output of $\mathcal{N}$ as a set of $|L|$ transformations $f_i(.), i \in \{1, ..., |L|\}$. For the sake of simplicity, each $f_i$ consists of a series of convolution, batch normalization, and activation operations. In this definition, we obtain the network output ($y$) by forwarding the input data, denoted by $X$, through the sequential layers $f$, where the input of layer $i$ is the output of the previous layer $i-1$; therefore, $y = f_{|L|}(...f_2(f_1(X)))$. This composes the idea behind plain networks (i.e., VGG and AlexNet). 

In residual-like networks, we can express the output $y_i$ of layer $i$ in terms of the transformation $f_i$ and the output $y_{i-1}$ from the previous layer (see Figure~\ref{fig:residualmodule} top). Formally, we write: %the output of the $i$-th layer as
\begin{equation}\label{eq:residual}
	y_i = f_i(y_{i-1}) + y_{i-1}.
\end{equation} 

Equation~\ref{eq:residual} composes a residual module, where the rightmost part is named \emph{identity-mapping shortcut} (or identity for short). From a theoretical perspective, pruning the $i$-th layer corresponds to letting $y_i = y_{i-1}$. 
%From a technical perspective, pruning the $i$-th layer consists of connecting the output of layer $i-1$ to the input of layer $i+1$. 
From a technical perspective, pruning the $i$-th layer involves connecting the output of layer $i-1$ to the input of layer $i+1$. Due to the residual nature (skip connection), we could accomplish this by just zeroing out the weights of $f_i(y_{i-1})$; thus, eliminating its contribution in Equation~\ref{eq:residual}. However, this process does not ensure practical speed-up without specialized hardware for sparse computing. Instead, after selecting a victim layer (let's say layer $i$), we obtain a pruned model according to the following process. First, we create a novel architecture without layer $i$, resulting in a model comprising only the surviving layers (the pruned model). Then, from the old architecture (unpruned model), we transfer the weights of the survival layers (we can apply this idea to a set of layers at once) to this novel architecture. Figure \ref{fig:residualmodule} (bottom) illustrates this process. 

From the process above, we highlight that the layer-pruning process removes building blocks (i.e., a set of transformations, $f_i(.)$) a.k.a modules. Therefore, the pruning also eliminates the corresponding activations and normalization layers from the block. This is a common process in layer-pruning techniques~\cite{Zhang&Liu:2022,Jordao:2020,Zhou:2022}.

As a final note, the pruning process cannot remove all layers composing a model due to incompatible dimensions between the input and output tensor between stages (layers operating on representations in the same resolution). In particular, the pruning is unable to remove layers between stages. Thus, given an architecture of $k$ layers within a stage, the pruning can remove at most $k-2$ layers within this stage. Importantly, this is the reason why we are unable to remove all layers of a model. This analysis corresponds to ResNet architecture and can vary depending on the architecture design of the model.
\begin{figure}[!!htb]
	\centering
	\includegraphics[width=\columnwidth]{Figures/Appendix/PruningLayers}
	\caption{Architecture of a residual-like network. Top. The rationale behind this architecture is that the output of a layer takes into account the transformation performed by it ($f$) plus ($\oplus$) the input ($y$) it receives. Due to this essence, when we disable layer $i$ (its transformation -- dashed lines), the output (representation) of layer $i-1$ is propagated to layer $i+1$, which means that the output $y_i$ belongs $y_{i-1}$. For the sake of simplicity, we omit the batch normalization and activation layers, which are also transferred in the process of layer removal. Bottom. Process to eliminate a layer from a technical perspective and, thus, obtain practical speed-up gains. After selecting the victim layer (i.e., Layer $i$), we create a novel architecture without it and, then, transfer the weights (red dashed arrows) of the corresponding survival layers.}
	\label{fig:residualmodule}
\end{figure}
\subsection{Adversarial Attacks}\label{sec:adv_att}
\begin{figure}[!t]
	\centering
	\includegraphics[width=0.48\columnwidth]{Figures/Appendix/CIFAR10_2_deltas.pdf}
	\includegraphics[width=0.48\columnwidth]{Figures/Appendix/mEC_deltas.pdf}
	\includegraphics[width=0.48\columnwidth]{Figures/Appendix/FGSM_deltas.pdf}
	\includegraphics[width=0.48\columnwidth]{Figures/Appendix/ImageNetC_deltas.pdf}
	\caption{Results of pruned models for different adversarial attacks. Green and blue points correspond to an accuracy improvement and degradation, respectively. Dotted lines separate the plots into improvement and degradation groups. Top-Right: Results on out-of-distribution using CIFAR-10.2~\cite{Lu:2020}. Top-Left: Results on adversarial robustness using CIFAR-C~\cite{Hendrycks:2019}. Bottom: Results on FGSM adversarial attack.}
	\label{fig:Adv_deltas}
\end{figure}
Efforts toward a deeper understanding of the roles played by layers in network generalization and the effect of pruning in adversarial attack scenarios reinforce the idea that improving  OOD and adversarial robustness while reducing computational demand is accomplishable for pruning methods~\cite{Masarczyk:2023,Bair:2024}. Such compromises are crucial for deploying these models in safety-critical applications e.g., autonomous driving and robotics. In this experiment, we demonstrate that our pruned models improve OOD generalization and adversarial robustness. For this purpose, we compare the performance on different adversarial tasks of ResNet56 and its pruned models using our method. Figure~\ref{fig:Adv_deltas} shows the results. According to this figure, our pruned models obtain positive robustness, highlighting their effectiveness even on severe compression rates. Specifically, on CIFAR-10.2~\cite{Lu:2020} and CIFAR-C~\cite{Hendrycks:2019}, we reduce more than 70\% of computational cost while exhibiting improvements. Notably, only three pruned models obtained lower performance compared to the unpruned model, yet less than one pp. In the FGSM attack, regardless of the FLOP reduction levels, our pruned models dominate its unpruned version in terms of robustness. 
	
It is worth mentioning that during the pruning process, we avoid any defense mechanism. Therefore, the preceding discussion confirms that the benefits of our pruned models extend beyond computational gains.

\subsection{Results on Shallow Architectures}\label{sec:sup_tables}
Regarding residual architectures, Table~\ref{tab:resnet32:resnet44} shows that our method removes up to $54.61\%$ and $62.95\%$ of FLOPs without compromising accuracy. At higher compression rates, the performance drop is negligible (i.e., less than one pp.). These results align with our discussion considering deep models and reinforce the effectiveness of our method on shallow architectures.

Compared to the state-of-the-art, we outperform all methods except for the one by Nonnenmacher et al.~\cite{Nonnemacher:2022} on ResNet32. Due to the shallowness of the architecture, our method reached the limit of layer removal (i.e., there are no more available layers to prune). See Section~\ref{sec:technical_issues}. To further achieve computational gains, we combine our method with filter-pruning strategies.

Finally, few methods appear in this table due to the lack of pruning studies that report results on these architectures~\cite{He:2023}.
\begin{table}[!t]
	\centering
	\small
	
	\caption{Comparison of state-of-the-art pruning methods on CIFAR-10 using ResNet32 and ResNet44. The symbols (+) and (-) denote increase and decrease in accuracy regarding the original (unpruned) network, respectively. For each level of FLOP reduction, we highlight the best results in bold.}
	\label{tab:resnet32:resnet44}
\begin{tabular}{llrc}
	\hline
	& Method                             & $\Delta$ Acc.     & FLOPs (\%)     \\ \hline
	\multicolumn{1}{l|}{\multirow{8}{*}{ResNet32}} & GKP-TMI~\cite{Zhong:2022} (ICLR, 2022)    & (+)0.22           & 43.10 \\
	\multicolumn{1}{l|}{} & SOKS~\cite{Liu:2023} (TNNLS, 2023) & (-) 0.38          & 46.85          \\
	\multicolumn{1}{l|}{} & CKA (ours)                         & \textbf{(+) 0.68} & \textbf{47.78} \\ \cline{2-4} 
	\multicolumn{1}{l|}{}                          & DAIS~\cite{Guan:2023} (TNNLS, 2023)       & \textbf{(+) 0.57} & 53.90 \\
	\multicolumn{1}{l|}{} & SOKS~\cite{Liu:2023} (TNNLS, 2023) & (-) 0.80          & 54.58          \\
	\multicolumn{1}{l|}{} & CKA (ours)                         & (+) 0.05          & \textbf{54.61} \\ \cline{2-4} 
	\multicolumn{1}{l|}{}                          & SOSP~\cite{Nonnemacher:2022} (ICLR, 2022) & (-) 0.24          & \textbf{67.36} \\
	\multicolumn{1}{l|}{} & CKA (ours)                         & \textbf{(-) 0.18} & 61.44 \\ \hline
	\multicolumn{1}{l|}{\multirow{5}{*}{ResNet44}} & DCP-CAC (TNNLS, 2022)                     & (-) 0.03          & 50.04 \\
	\multicolumn{1}{l|}{} & AGMC (ICCV, 2021)                  & (-) 0.82          & 50.00          \\
	\multicolumn{1}{l|}{} & CKA (ours)                         & \textbf{(+) 0.47} & \textbf{53.27} \\ \cline{2-4} 
	\multicolumn{1}{l|}{} & CKA (ours)                         & (+) 0.22          & 62.95          \\
	\multicolumn{1}{l|}{} & CKA (ours)                         & (-) 0.29          & 72.64          \\ \hline
	\multicolumn{1}{l|}{\multirow{4}{*}{MobileNetV2}} & CKA (ours)  & (+) 0.17	& 26.60 \\
	\multicolumn{1}{l|}{}							 & CKA (ours)	& (-) 0.37	& 31.28 \\
	%\multicolumn{1}{l|}{}							& CKA (ours) + $\ell_1$ & (-) 0.70 & 51.01 \\
	%\multicolumn{1}{l|}{}							& CKA (ours) + $\ell_1$ & (-) 1.45 & 73.89 \\
	\multicolumn{1}{l|}{}							& CKA (ours) + $\ell_1$ & (-) 2.82 & 82.89 \\
	\multicolumn{1}{l|}{}							& CKA (ours) + $\ell_1$ & (-) 3.44 & 85.06 \\ \hline
\end{tabular}
\end{table}

\subsection{Results on Transformer Architecture}\label{sec:transformer}
Recent advancements in foundation models and general-purpose tasks frequently rely on Transformer architectures and their variants.

In the context of layer-pruning, Dong et al.~\cite{Dong:2021} noted that Transformer-like architectures exhibit analogous behavior to ResNets --  they experience either no degradation or only negligible drops in accuracy when removing certain layers. Such a claim provides a guarantee to perform layer-pruning on these architectures.

In this experiment, we evaluate the effectiveness of our layer-pruning method on the widely used Transformer architecture. Unfortunately, our limited computational budget prevents us from considering Visual Transformers, which typically require thousands of samples (e.g., JFT-300M) to achieve competitive results compared to convolutional networks. Thereby, we assess our layer-pruning technique in Transformers for human activity recognition based on wearable sensors, a popular application involving tabular data. Details about these datasets are available at this link: \emph{https://doi.org/10.1016/j.neucom.2020.04.151}.

Our Transformer architecture (unpruned) comprises $10$ layers, each with $128$ heads and projection dimensions of $64$. For each dataset, we train this Transformer architecture for $200$ epochs and subsequently prune it similarly to the approach described in the main body of the paper. We emphasize that our objective here is not to advance the state-of-the-art; rather, we aim to demonstrate that the effectiveness of our layer-pruning extends beyond ResNet architectures.

Figure~\ref{fig:transformer} shows the results. In this figure, the black dashed line shows where the drop in accuracy is zero; hence, pruned models (green points) above this line exhibit an accuracy improvement. From Figure~\ref{fig:transformer}, we observe that most pruned models exhibited no accuracy drop, even on high compression regimes. Therefore, we conjecture that on these datasets the layer-pruning technique operated as a strong regularization mechanism. We observe that the regularization performs well as a function of the dataset size. For example, the datasets on the upper side of Figure~\ref{fig:transformer} are at least 3 times smaller (in terms of training size) compared to the ones on the lower side. We intend to further explore this behavior in future research, particularly in low-data regimes, which is a well-known deficit in Transformer-like architectures.
%UTD-MHAD2 = (795, 25)
%WHARF = (2709, 13)
%USCHAD = (6876, 25)
%PAMAP2P = (5265, 157)
In summary, the results of this experiment confirm the effectiveness of our layer-pruning method on the Transformer architecture for tabular data.

\begin{figure}[!t]
	\centering
	\includegraphics[width=0.45\linewidth]{Figures/Appendix/UTD-MHAD2_1s}
	\includegraphics[width=0.45\linewidth]{Figures/Appendix/WHARF}
	\includegraphics[width=0.45\linewidth]{Figures/Appendix/USCHAD}
	\includegraphics[width=0.45\linewidth]{Figures/Appendix/PAMAP2P}
	\caption{Performance of our layer-pruning method on Transformer architecture for human activity recognition based on wearable sensors (tabular data). Each point denotes a pruned model and the black-dashed line indicates the point where the drop in accuracy is zero; thus, points above this line (green) stand for pruned models with an improved accuracy compared to the original, unpruned, model.}
	\label{fig:transformer}
\end{figure}
